# Supplementary material for: Perspective picture from Visual Sphere: a new approach to image rasterization
Source: arXiv:2003.10558 ancillary file (2020-10-18)
Supplement: Supplementary file 1 [file Example-Perspective_Map_Rasterization-JM_Fober.pdf]

# Perspective map rasterization

by Jakub Max Fober, learn more on <http://maxfober.space/> or contact [talk@maxfober.space](mailto:talk@maxfober.space)

January 29  
2020

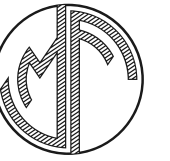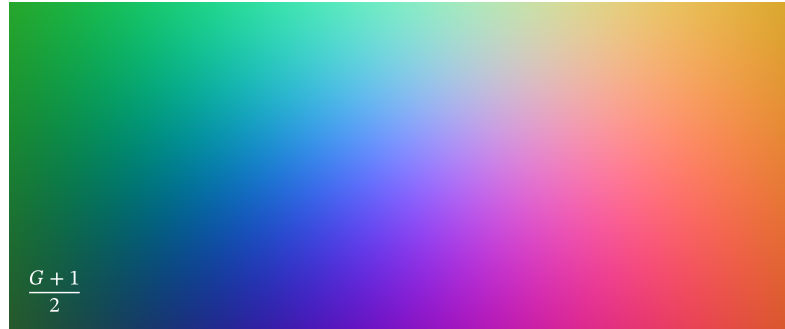

Perspective map source format of some type projection

M  
a  
p

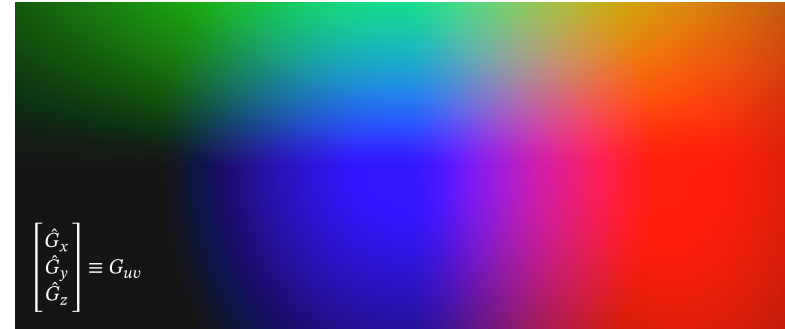

Visual-sphere texture map G representing unit vectors in range  $[-1, 1]^3$

M  
a  
p

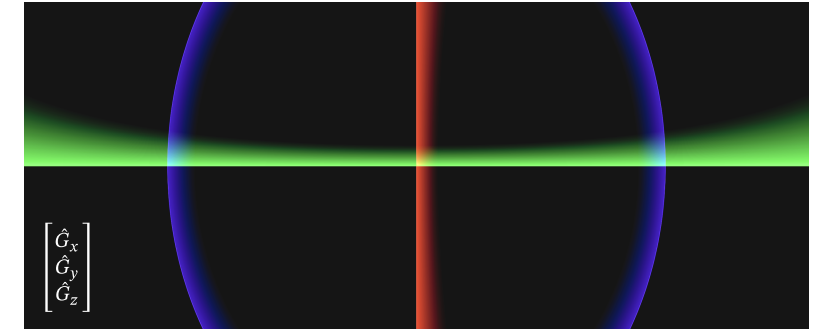

Visualization of visual-sphere texture axis position 0

$\vec{A}$   
 $\vec{B}$   
 $\vec{C}$

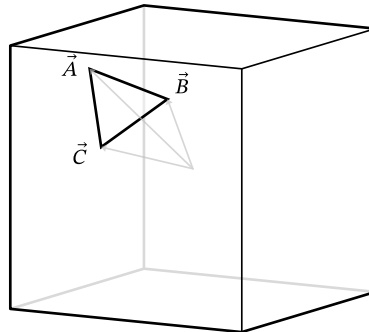

Triangle in clip space

V  
e  
r  
t  
e  
x

$$\begin{bmatrix} \|\vec{A} \times \vec{B}\| \\ \|\vec{B} \times \vec{C}\| \\ \|\vec{C} \times \vec{A}\| \end{bmatrix}$$

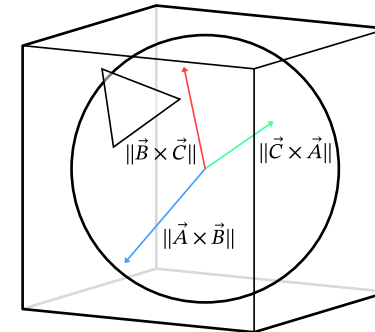

Triangle rasterization matrix

V  
e  
r  
t  
e  
x

$$\begin{aligned} a^2 &= |\vec{B} - \vec{C}|^2 \\ b^2 &= |\vec{C} - \vec{A}|^2 \\ c^2 &= |\vec{A} - \vec{B}|^2 \\ \begin{bmatrix} \vec{O}_s \\ \vec{O}_t \\ \vec{O}_p \end{bmatrix} &= \begin{bmatrix} a^2(b^2 + c^2 - a^2) \\ b^2(c^2 + a^2 - b^2) \\ c^2(a^2 + b^2 - c^2) \end{bmatrix} \\ \vec{S} &= \begin{cases} 0.5(\vec{B} + \vec{C}), & \text{if } \vec{O}_s \leq 0 \\ 0.5(\vec{C} + \vec{A}), & \text{if } \vec{O}_t \leq 0 \\ 0.5(\vec{A} + \vec{B}), & \text{if } \vec{O}_p \leq 0 \\ \frac{\vec{O}_s \vec{A} + \vec{O}_t \vec{B} + \vec{O}_p \vec{C}}{\vec{O}_s + \vec{O}_t + \vec{O}_p}, & \text{otherwise} \end{cases} \blacksquare \end{aligned}$$

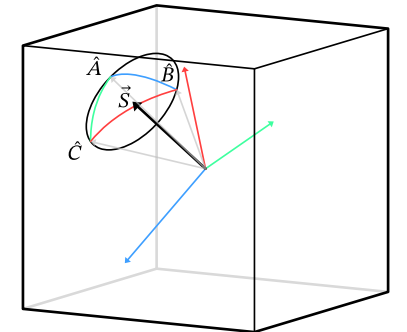

Center of the smallest circle over triangle

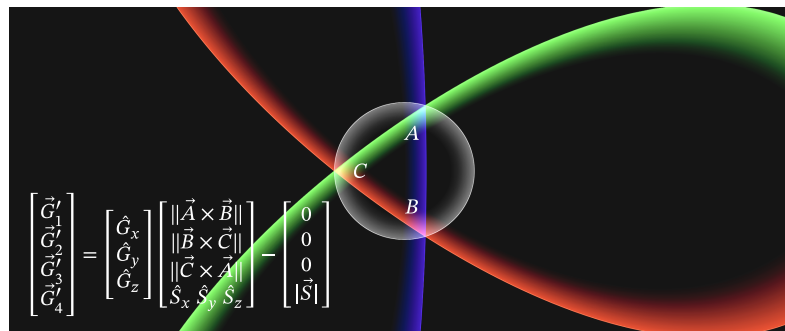

Visualization of rotated perspective map  $G'$

F  
r  
a  
g  
m  
e  
n  
t

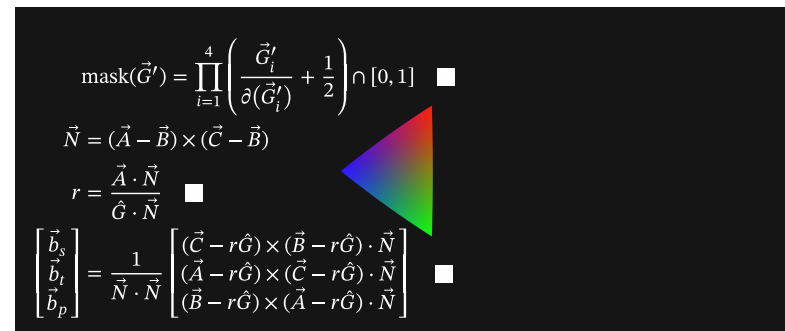

Rasterized triangle with barycentric coordinates and distance occlusion mask

F  
r  
a  
g  
m  
e  
n  
t

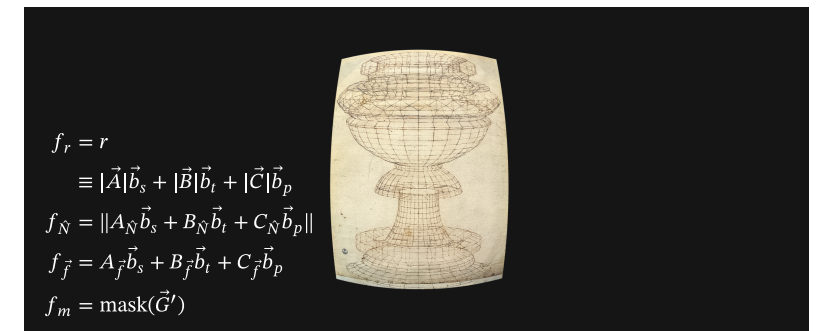

Fragment data interpolation of model with texture (Paolo Uccello, 15<sup>th</sup> century)

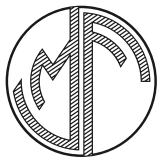

# Various perspective maps

by Jakub Max Fober, learn more on <http://maxfober.space/> or contact [talk@maxfober.space](mailto:talk@maxfober.space)

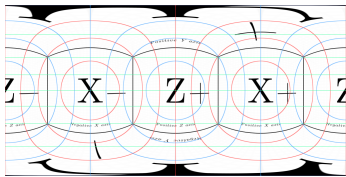

$$\begin{bmatrix} \vec{f}'_x \\ \vec{f}'_y \end{bmatrix} = \frac{2\pi}{\pi} \left( \begin{bmatrix} \vec{f}_x \\ \vec{f}_y \end{bmatrix} - \begin{bmatrix} 0.5 \\ 0 \end{bmatrix} \right)$$

$$\begin{bmatrix} \hat{v}_x \\ \hat{v}_y \\ \hat{v}_z \end{bmatrix} = \begin{bmatrix} \sin(\vec{f}'_x) \\ -1 \\ \cos(\vec{f}'_x) \end{bmatrix} \begin{bmatrix} \sin(\vec{f}'_y) \\ \cos(\vec{f}'_y) \end{bmatrix}$$

Where  $\vec{f}$  is the texture coordinate vector and  $\vec{v}$  is the visual sphere vector.

360° equirectangular perspective map

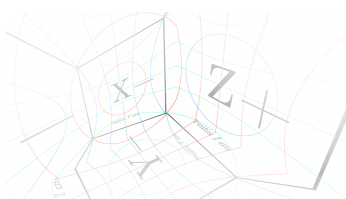

$$\begin{bmatrix} \hat{v}_x \\ \hat{v}_y \\ \hat{v}_z \end{bmatrix} = \left\| \begin{bmatrix} \vec{S}_x - \vec{O}_x \\ \vec{S}_y - \vec{O}_y \\ \vec{S}_z - \vec{O}_z \end{bmatrix} \begin{bmatrix} O_{11} & O_{12} & O_{13} \\ O_{21} & O_{22} & O_{23} \\ O_{31} & O_{32} & O_{33} \end{bmatrix} \right\|$$

$$m = \left( \frac{r}{\max(r)} \right)^2$$

Where  $\mathbf{O}$  is the observation point matrix, vector  $\mathbf{O}$  is the observation point position,  $\mathbf{S}$  vector is the environment model surface position and  $\vec{v}$  is the visual sphere vector as environment surface color.  $m$  is the light dimming mask, where  $r$  is the distance pass. Environment is photographed from projection position.

Projection mapping environment map

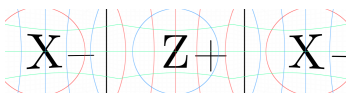

$$i = \left\lfloor n \vec{f}_x \right\rfloor + \frac{1-n}{2}$$

$$\begin{bmatrix} \hat{v}_x \\ \hat{v}_y \\ \hat{v}_z \end{bmatrix} = \left\| \begin{bmatrix} \text{fract}(n \vec{f}_x) 2 - 1 \\ (2 \vec{f}_y - 1) n \div a \\ \cot \frac{\Omega}{2} \end{bmatrix} \begin{bmatrix} \cos(i\Omega) & 0 & \sin(i\Omega) \\ 0 & 1 & 0 \\ -\sin(i\Omega) & 0 & \cos(i\Omega) \end{bmatrix} \right\|$$

Where  $n$  is the number of screens,  $a$  and  $\Omega$  are the single-screen aspect ratio and horizontal FOV respectively,  $\vec{f}$  is the texture coordinate vector and  $\vec{v}$  is the visual sphere vector.

$n$  - screen horizontal array perspective map

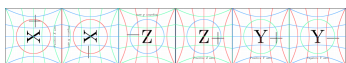

$$\begin{aligned} \hat{X} &= [1, 0, 0] \\ \hat{Y} &= [0, 1, 0] \\ \hat{Z} &= [0, 0, 1] \end{aligned}$$

Where  $\vec{f}$  is the texture coordinate vector and  $\vec{v}$  is the visual sphere vector.

$$i = \left\lfloor 6 \vec{f}_x \right\rfloor$$

$$\begin{bmatrix} \hat{v}_x \\ \hat{v}_y \\ \hat{v}_z \end{bmatrix} = \left\| \begin{bmatrix} \text{fract}(6 \vec{f}_x) - 1/2 \\ \vec{f}_y - 1/2 \\ 1/2 \end{bmatrix} \begin{cases} [\hat{Z}, -\hat{X}, -\hat{Y}], & \text{if } i = 0 \\ [-\hat{Z}, \hat{X}, -\hat{Y}], & \text{if } i = 1 \\ [\hat{X}, -\hat{Y}, -\hat{Z}], & \text{if } i = 2 \\ [\hat{X}, \hat{Z}, -\hat{Y}], & \text{if } i = 4 \\ [-\hat{X}, -\hat{Z}, -\hat{Y}], & \text{if } i = 5 \end{cases} \right\|$$

6x1 cubemap perspective map

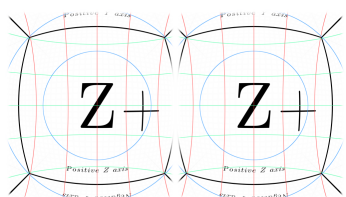

$$i = \text{sign}(2 \vec{f}_x - 1)$$

$$\begin{bmatrix} \vec{f}'_x \\ \vec{f}'_y \end{bmatrix} = \left( \begin{bmatrix} 2 \text{fract}(2 \vec{f}_x) - 1 \\ 2 \vec{f}_y - 1 \end{bmatrix} + \begin{bmatrix} i(1-2d) \\ 0 \end{bmatrix} \right) \begin{bmatrix} 0.5a \\ 1 \end{bmatrix}$$

$$\begin{bmatrix} \vec{f}''_x \\ \vec{f}''_y \end{bmatrix} = \begin{bmatrix} \vec{f}'_x \\ \vec{f}'_y \end{bmatrix} \frac{1 + k_1 |\vec{f}'|^2 + k_2 |\vec{f}'|^4 + \dots + k_n |\vec{f}'|^{2n}}{1 + k_1 + k_2 + \dots + k_n}$$

$$\begin{bmatrix} \hat{v}_x \\ \hat{v}_y \\ \hat{v}_z \end{bmatrix} = \left\| \begin{bmatrix} \vec{f}''_x \\ \vec{f}''_y \\ \cot \frac{\Omega}{2} \end{bmatrix} \right\|$$

Where  $d$  is the IPD in screen-width,  $a$  is the screen aspect ratio,  $\Omega$  is the vertical FOV,  $k_1$  and  $k_2$  are the lens-distortion coefficients,  $\vec{f}$  is the texture coordinate vector and  $\vec{v}$  is the visual sphere vector.

Simple VR perspective map

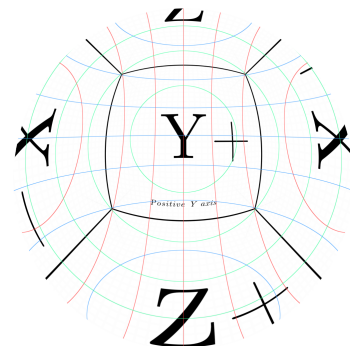

$$\begin{bmatrix} \vec{f}'_x \\ \vec{f}'_y \end{bmatrix} = \begin{bmatrix} 2 \vec{f}_x - 1 \\ 1 - 2 \vec{f}_y \end{bmatrix}$$

$$\theta = |\vec{f}'| \left( \Omega + \frac{\pi}{2} \right)$$

$$\begin{bmatrix} \hat{v}_x \\ \hat{v}_y \\ \hat{v}_z \end{bmatrix} = \left\| \begin{bmatrix} \vec{f}'_x \sin \theta \div |\vec{f}'| \\ \cos \theta \\ o + \vec{f}'_y \sin \theta \div |\vec{f}'| \end{bmatrix} \begin{bmatrix} 1 & 0 & 0 \\ 0 & \cos \varphi & -\sin \varphi \\ 0 & \sin \varphi & \cos \varphi \end{bmatrix} \right\|$$

$$m = \frac{1 - |\vec{f}'|}{\Delta(1 - |\vec{f}'|)} \cap [0, 1]$$

Where  $\vec{f}$  is the texture coordinate vector and  $\vec{v}$  is the visual sphere vector,  $m$  is the radial mask,  $\varphi$  is the tilt angle and  $\Omega$  is the compression angle.  $\Delta$  is the  $f$ width function and  $o$  is the view position offset in radius.

Full dome

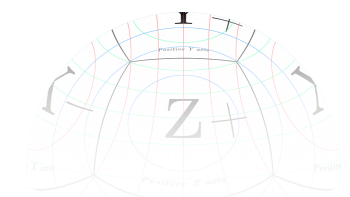

$$\vec{I} = \hat{N} - \vec{P}$$

$$\hat{R} = \|\vec{I} - 2(\vec{I} \cdot \hat{N})\hat{N}\|$$

$$r = \hat{R} \cdot (\vec{O} - \vec{N})$$

$$r' = r + \sqrt{d^2 - |r\hat{R} + \hat{N} - \vec{O}|^2}$$

$$\hat{v} = \|r'\hat{R} + \hat{N} - \vec{O}\|$$

$$m = \left( \frac{r' + |\vec{I}|}{\max(r' + |\vec{I}|)} \right)^2$$

Where  $\vec{v}$  is the visual sphere vector as mirror surface color,  $\hat{N}$  is the spherical mirror surface position,  $\vec{P}$  is the projector position and  $\mathbf{O}$  is the dome origin position with  $d$  as the dome radius. Mirror radius is equal 1 with its origin at position  $(0, 0)$ . Light-dimming mask is denoted by  $m$ , based on inverse-square law approximation.

Spherical mirror dome reflection color

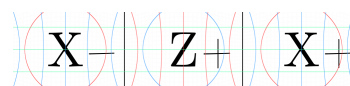

$$a = \frac{\Omega}{h}$$

$$\begin{bmatrix} \vec{f}'_x \\ \vec{f}'_y \end{bmatrix} = \begin{bmatrix} \Omega \\ h \end{bmatrix} \left( \begin{bmatrix} \vec{f}_x \\ \vec{f}_y \end{bmatrix} - \frac{1}{2} \right)$$

$$\begin{bmatrix} \hat{v}_x \\ \hat{v}_y \\ \hat{v}_z \end{bmatrix} = \left\| \begin{bmatrix} \sin(\vec{f}'_x) \\ \vec{f}'_y \\ \cos(\vec{f}'_x) \end{bmatrix} \right\|$$

Where  $a$  is the image aspect ratio,  $h$  is the display height-to-radius proportion,  $\vec{f}$  is the texture coordinate vector and  $\vec{v}$  is the visual sphere vector,  $\Omega$  is the horizontal field of view of the display.

Curved panorama

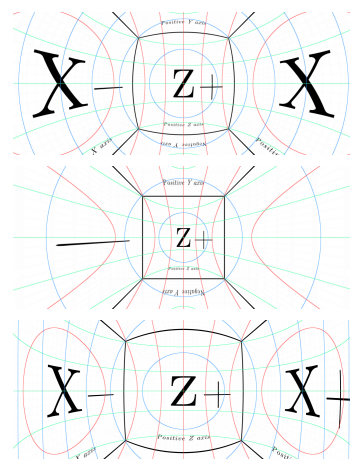

$$\vec{f}'_x = \begin{cases} 2 \vec{f}_x - 1, & \text{if } \Omega^h \\ a(2 \vec{f}_x - 1), & \text{if } \Omega^v \\ a(2 \vec{f}_x - 1) \div \sqrt{a^2 + 1}, & \text{if } \Omega^d \end{cases}$$

$$\vec{f}'_y = \begin{cases} (2 \vec{f}_y - 1) \div a, & \text{if } \Omega^h \\ 2 \vec{f}_y - 1, & \text{if } \Omega^v \\ (2 \vec{f}_y - 1) \div \sqrt{a^2 + 1}, & \text{if } \Omega^d \end{cases}$$

$$R = \sqrt{\vec{f}_x'^2 + l \vec{f}_y'^2}$$

$$\theta = \begin{cases} \arctan(\tan(k \frac{\Omega}{2}) R) \div k, & \text{if } 0 < k \leq 1 \\ R \frac{\Omega}{2}, & \text{if } k = 0 \\ \arcsin(\sin(k \frac{\Omega}{2}) R) \div k, & \text{if } 0 > k \geq -1 \end{cases}$$

$$\begin{bmatrix} \hat{v}_x \\ \hat{v}_y \\ \hat{v}_z \end{bmatrix} = \left\| \begin{bmatrix} \vec{f}'_x/R \\ \vec{f}'_y/R \\ 1 \end{bmatrix} \begin{bmatrix} \sin \theta \\ \sin \theta \div (s + (1-s)l) \\ \cos \theta \end{bmatrix} \right\|$$

Where  $\vec{f}$  is the texture coordinate vector,  $\vec{v}$  is the visual sphere vector,  $a$  is the aspect ratio and  $\Omega$  is the field of view angle.  $k$  is the projection coefficient,  $l$  is the cylindrical projection factor and  $s$  is anamorphic correction of cylindrical projection.

$k = -1$  is orthographic  
 $k = 0.5$  is equisolid  
 $k = 0$  is equidistant  
 $k = 0.5$  is stereographic  
 $k = 1$  is rectilinear  
 $l \in (0, 1]$  cylindrical-spherical  
 $s \in [0.8, 1]$

Universal perspective
